# Supplementary material for: ARAUS: A Large-Scale Dataset and Baseline Models of Affective Responses to Augmented Urban Soundscapes
Source: arXiv:2207.01078 source file (2024-07-02)
Supplement: Supplementary file 7 [file cnn_architecture.tex]

\begin{figure}[t]
	\centering
	\includegraphics[width=0.82\linewidth]{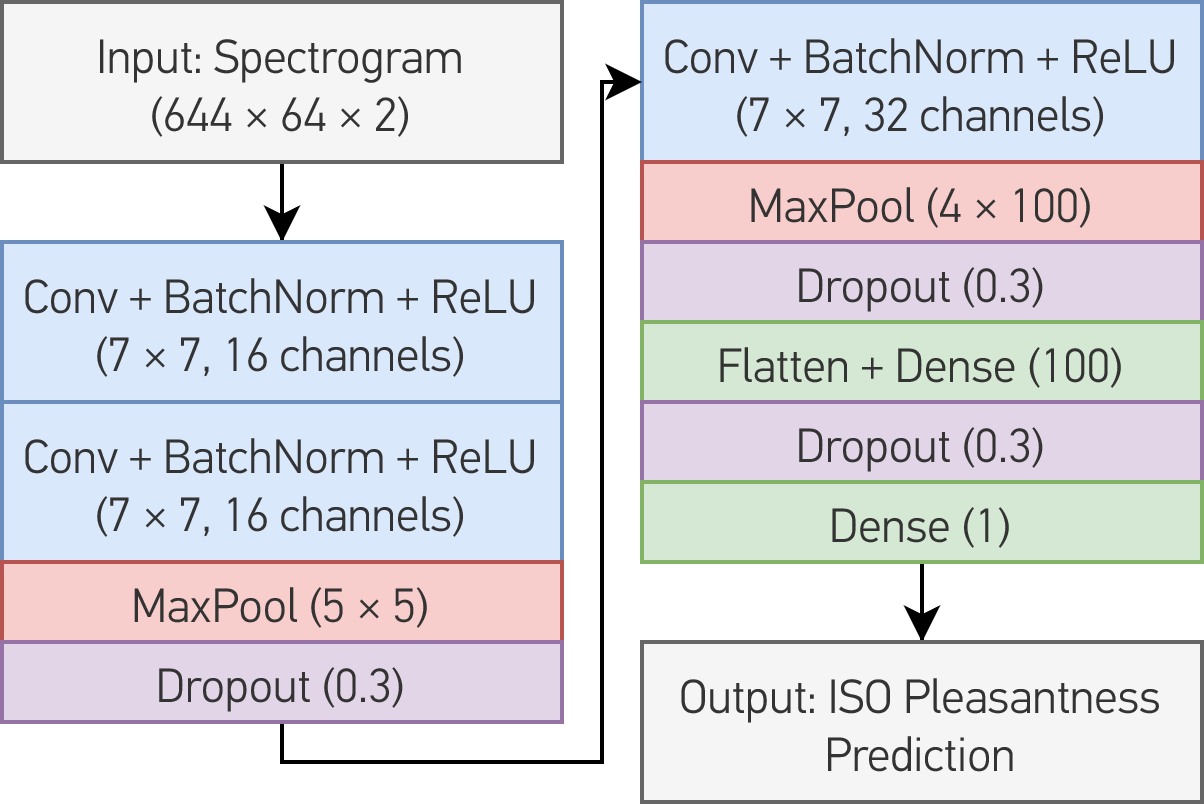}
	\caption{Baseline CNN model architecture, adapted from \cite{Heittola2020AcousticSolutions}}
	\label{fig:CNN Architecture}
\end{figure}
