# Supplementary material for: ARAUS: A Large-Scale Dataset and Baseline Models of Affective Responses to Augmented Urban Soundscapes
Source: arXiv:2207.01078 source file (2024-07-02)
Supplement: Supplementary file 13 [file rooms.tex]

\begin{figure}[t]
	\centering
	\includegraphics[width=0.49\columnwidth]{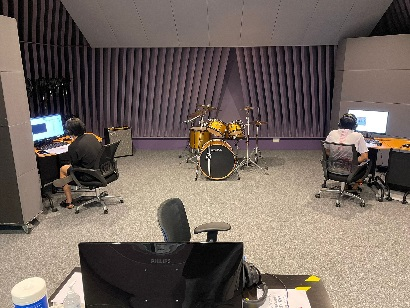} 
	\includegraphics[width=0.49\columnwidth]{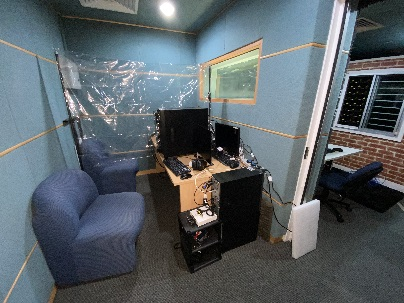} 
	\includegraphics[width=0.49\columnwidth]{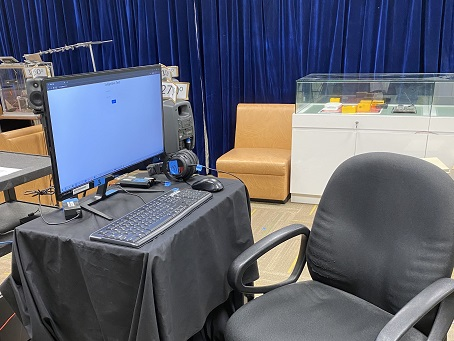} 
	\includegraphics[width=0.49\columnwidth]{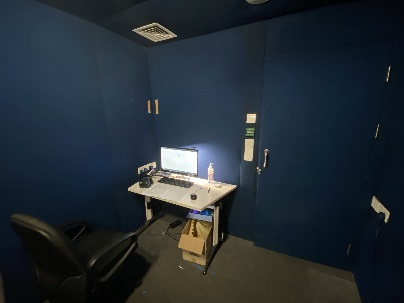} 
	\caption{Test sites at (top left) Academic Media Studio, SUTD, (top right) Media Technology Laboratory, NTU, (bottom left) Demo Room, NTU, (bottom right) Interactive Soundscape Room, NTU. Their noise floors, measured as $L_{\text{A,eq,3-min}}$ values with a B\&K Sound Level Meter Type 2240, were \SI{20.6}{\decibel}, \SI{26.0}{\decibel}, \SI{36.9}{\decibel}, and \SI{30.2}{\decibel}, respectively.}
	\label{fig:Rooms}
\end{figure}
