# Supplementary material for: ARAUS: A Large-Scale Dataset and Baseline Models of Affective Responses to Augmented Urban Soundscapes
Source: arXiv:2207.01078 source file (2024-07-02)
Supplement: Supplementary file 26 [file age_distribution.tex]

\begin{table}[t]
	\centering
	\caption{
		Age and gender\protect\footnotemark{} distribution of participants\\in ARAUS dataset by fold and in entirety.
		}
	\label{tab:age_distribution}
	
	\begin{tabularx}{\linewidth}{Xccccccc}
		\toprule
		& \multicolumn{6}{c}{Fold} & \\
		\cmidrule{2-7}
		Statistic        & Test &    1 &    2 &    3 &    4 &    5 &  All \\
		\midrule
		Sample size      &    5 &  120 &  120 &  120 &  120 &  120 &  605 \\
		\# female        &    4 &   62 &   56 &   69 &   68 &   69 &  328 \\   
		\# male          &    1 &   58 &   64 &   51 &   52 &   51 &  277 \\
		\midrule
		Mean age         & 22.4 & 27.4 & 26.7 & 26.3 & 27.3 & 26.3 & 26.7 \\
		Std. dev. of age &  5.5 & 10.2 &  9.8 & 10.4 & 11.0 &  8.7 & 10.0 \\
		Minimum age      &   18 &   19 &   18 &   18 &   18 &   18 &   18 \\
		Median age       &   21 &   24 &   24 &   23 &   23 &   24 &   24 \\
		Maximum age      &   32 &   63 &   71 &   68 &   65 &   60 &   71 \\
		\bottomrule
	\end{tabularx}
\end{table}

\footnotetext{To safeguard their identities, the small number (2 participants, \SI{0.33}{\percent})
% -- Kenneth, please check 
of participants identifying as neither male nor female were randomly assigned as ``male'' or ``female'' in the public release of the ARAUS dataset, each with a probability of \SI{50}{\percent}.}
